# Supplementary material for: What is Wrong with End-to-End Learning for Phase Retrieval?
Source: arXiv:2403.15448 source file (2024-03-18)
Supplement: Supplementary file 1 [file appendix.tex]

\section{Appendix -- Phase-Adjusted MSE}\label{app:pamse}

In this section we will briefly show how the phase-adjusted MSE is derived. Due to the intrinsic symmetries in the FFPR problem, we need to adjust the global phase before we evaluate the quality of the recovered images. Meanwhile, we need to scale the two images in the Error Function:
\begin{equation}  \label{eq:main}
  \min_{\mb \theta , \mb \eta>0} \; \norm{\mb A - \mb \eta \mb B \mb e^{i\mb \theta}}_{F}^2
\end{equation}
where $\mb A$ is the original image in the object domain and $\mb B$ is the recovered image in the object domain. $\mb \eta$ is scale variable and $\mb \theta$ is a global phase.

Then we could expand the objective function based on the complex-valued rule:
\begin{equation}  \label{eq:main1}
  \min_{ \mb \eta>0} \; \norm{\mb A}_{F}^2 + \norm {\mb \eta \mb B}_{F}^2 - 2 \mb \eta Real \paren{ \innerprod{\mb A}{\mb B \mb e^{i \mb \theta}}}
\end{equation}

which equals to :
\begin{equation}  \label{eq:main2}
  \min_{ \mb \eta>0} \; \norm{\mb A}_{F}^2 + \norm {\mb \eta \mb B}_{F}^2 - 2 \mb \eta |\innerprod{\mb A}{\mb B}|
\end{equation}

First-order optimal condition:
\begin{equation}
    \nabla _{ \mb \eta} \; \norm{\mb A}_{F}^2 + \norm {\mb \eta \mb B}_{F}^2 - 2 \mb \eta |\innerprod{\mb A}{\mb B}| = 0
\end{equation}
Deriving the objective function expansion form:
\begin{equation}
    2\mb \eta \norm{\mb B}_{F}^2 -2|\innerprod{\mb A}{\mb B}| = 0
\end{equation}
Solution of $\eta$ :
\begin{equation}
    \mb \eta = \frac{|\innerprod{\mb A}{\mb B}|}{\norm{\mb B}_{F}^2}
\end{equation}

After substituting solution of $\mb \eta$ , we can get our PA-MSE metric which is defined in the follow form:
\begin{equation}
    \text{PA-MSE}\paren{\mb A,\mb B} = \norm{\mb A}_{F}^2 - \frac{|\innerprod{\mb A}{\mb B}|^2}{\norm{\mb B}_{F}^2}
\end{equation}
